# Supplementary material for: Self-Contrastive Forward-Forward Algorithm
Source: arXiv:2409.11593 source file (2025-03-27)
Supplement: Supplementary file 1 [file supplementary.tex]

\documentclass[sn-mathphys-num]{sn-jnl}% Math and Physical Sciences Numbered Reference Style 
%%\documentclass[sn-mathphys-ay]{sn-jnl}% Math and Physical Sciences Author Year Reference Style
%%\documentclass[sn-aps]{sn-jnl}% American Physical Society (APS) Reference Style
%%\documentclass[sn-vancouver,Numbered]{sn-jnl}% Vancouver Reference Style
%%\documentclass[sn-apa]{sn-jnl}% APA Reference Style 
%%\documentclass[sn-chicago]{sn-jnl}% Chicago-based Humanities Reference Style

%%%% Standard Packages
%%<additional latex packages if required can be included here>

\usepackage{graphicx}%
\usepackage{multirow}%
\usepackage{amsmath,amssymb,amsfonts}%
\usepackage{amsthm}%
\usepackage{mathrsfs}%
\usepackage{makecell}
\usepackage[title]{appendix}%
\usepackage{xcolor}%
\usepackage{textcomp}%
\usepackage{manyfoot}%
\usepackage{booktabs}%
\usepackage{algorithm}%
\usepackage{algorithmicx}%
\usepackage{algpseudocode}%
\usepackage{listings}%
\usepackage{comment}
\usepackage{amssymb}
\usepackage{pgfplots}
\pgfplotsset{compat=1.18}
\usepackage{array}
\usepackage{tabularx}
\usepackage{tabulary}
\usepackage{pifont}
\usepackage{tikz}
\usepackage{threeparttable}
\usepackage{subcaption}
\usepackage{listings}
\usepackage{xcolor} % for custom colors
\lstset{
  language=Python,               % Set language
  basicstyle=\ttfamily\footnotesize, % Basic font style
  keywordstyle=\color{blue},     % Keywords in blue
  commentstyle=\color{green!50!black}, % Comments in green
  stringstyle=\color{orange},    % Strings in orange
  showstringspaces=false,        % Don't show spaces in strings
  breaklines=true,               % Break long lines
  frame=single,                  % Frame around the code
  numbers=left,                  % Line numbers on the left
  numberstyle=\tiny\color{gray}, % Line number style
}

%\usepackage[backend=biber]{biblatex}
%\addbibresource{sn-bibliography.bib} % Main bibliography file
%\addbibresource{bib-ap.bib} % 

\usepackage{xcolor,pifont}
\newcommand*\colourcheck[1]{%
  \expandafter\newcommand\csname #1check\endcsname{\textcolor{#1}{\ding{52}}}%
}
\colourcheck{blue}
\colourcheck{green}
\colourcheck{red}

\newcommand*\colourcross[1]{%
  \expandafter\newcommand\csname #1cross\endcsname{\textcolor{#1}{\ding{55}}}%
}
\colourcross{blue}
\colourcross{green}
\colourcross{red}
%%%%

%%%%%=============================================================================%%%%
%%%%  Remarks: This template is provided to aid authors with the preparation
%%%%  of original research articles intended for submission to journals published 
%%%%  by Springer Nature. The guidance has been prepared in partnership with 
%%%%  production teams to conform to Springer Nature technical requirements. 
%%%%  Editorial and presentation requirements differ among journal portfolios and 
%%%%  research disciplines. You may find sections in this template are irrelevant 
%%%%  to your work and are empowered to omit any such section if allowed by the 
%%%%  journal you intend to submit to. The submission guidelines and policies 
%%%%  of the journal take precedence. A detailed User Manual is available in the 
%%%%  template package for technical guidance.
%%%%%=============================================================================%%%%

%% as per the requirement new theorem styles can be included as shown below
\theoremstyle{thmstyleone}%
%  meant for continuous numbers
%%\newtheorem{theorem}{Theorem}[section]% meant for sectionwise numbers
%% optional argument [theorem] produces theorem numbering sequence instead of independent numbers for Proposition
% 
%%\newtheorem{proposition}{Proposition}% to get separate numbers for theorem and proposition etc.

\theoremstyle{thmstyletwo}%

\theoremstyle{thmstylethree}%

\raggedbottom
%%\unnumbered% uncomment this for unnumbered level heads

\title[Article Title]{Self-Contrastive Forward-Forward Algorithm}

%%=============================================================%%
%% GivenName	-> \fnm{Joergen W.}
%% Particle	-> \spfx{van der} -> surname prefix
%% FamilyName	-> \sur{Ploeg}
%% Suffix	-> \sfx{IV}
%% \author*[1,2]{\fnm{Joergen W.} \spfx{van der} \sur{Ploeg} 
%%  \sfx{IV}}\email{iauthor@gmail.com}
%%=============================================================%%

%%%%%%%%%%%%%%%%%%%%%%
\author*[1]{\fnm{Xing} \sur{Chen}}\email{xing.chen@cnrs-thales.fr}

\author[1]{\fnm{Dongshu} \sur{Liu}}\email{dongshu.liu@cnrs.fr}

\author[2,3]{\fnm{J\'er\'emie} \sur{Laydevant}}\email{jeremie.laydevant@gmail.com}

\author*[1]{\fnm{Julie} \sur{Grollier}}\email{julie.grollier@cnrs-thales.fr}

\affil*[1]{\orgdiv{Laboratoire Albert Fert}, \orgname{CNRS, Thales, Universit\'e Paris-Saclay}, \orgaddress{\street{1 av. A. Fresnel}, \city{Palaiseau}, \postcode{91767},  \country{France}}}

\affil[2]{\orgdiv{School of Applied and Engineering Physics}, \orgname{Cornell University}, \orgaddress{\city{ Ithaca}, \postcode{NY 14853}, \country{USA}}}

\affil[3]{\orgdiv{USRA Research}, \orgname{Institute for Advanced Computer Science}, \orgaddress{\city{Mountain View}, \postcode{CA 94035}, \country{USA}}}
\end{comment}

%%==================================%%
%% Sample for unstructured abstract %%
%%==================================%%

\newpage
\begin{appendices}
\setcounter{page}{1}

\setcounter{figure}{0}
\setcounter{table}{0}
\setcounter{equation}{0}
\setcounter{algorithm}{0}

\section{On the convergence of $W_1$ and $W_2$}\label{app-converge}

The loss function of the SCFF method for one pair of positive input and negative input examples in the first layer (the layer index is neglected here) is defined as

\begin{equation}
    \ell_{i,j} = \text{log}(1+ \text{exp}(\Theta - ||\boldsymbol{y}_{i,\text{pos}}
 ||^2)) + \text{log}(1+ \text{exp}(||\boldsymbol{y}_{j,\text{neg}}||^2 - \Theta)) 
\end{equation}
where $||\boldsymbol{y}_{i,\text{pos}}
 ||^2$ and $||\boldsymbol{y}_{j,\text{neg}}||^2$ represent sum of the square of neuron activations respectively. The same procedure applies if mean activations are used instead. For simplicity, both threshold values $\Theta_{\text{pos}}$ and $\Theta_{\text{neg}}$ are assumed to be equal, i.e., $\Theta = \Theta_{\text{pos}} = \Theta_{\text{neg}}$. However, the same conclusion holds even if different thresholds are assumed for the positive and negative examples.
 $\boldsymbol{y}_{i,\text{pos}}$ and $\boldsymbol{y}_{j,\text{neg}}$ are calculated as
\begin{align}
    \boldsymbol{y}_{i,\text{pos}} &= f(W_1 \boldsymbol{x}_{k} + W_2 \boldsymbol{x}_{k}) \\
    \boldsymbol{y}_{j,\text{neg}} &= f(W_1 \boldsymbol{x}_{k} + W_2 \boldsymbol{x}_{n})
\end{align}

where $\boldsymbol{x}_k$ is a randomly selected example, and $\boldsymbol{x}_n$ is assumed to come from a different class of $\boldsymbol{x}_k$. $f$ is the ReLU activation function. 

The derivative of $\ell_{i,j}$ with respect to $W_1$ and $W_2$ are respectively

\begin{align}
    \frac{\partial \ell_{i,j}}{\partial W_1} &= \frac{-\text{exp}(\Theta - ||\boldsymbol{y}_{i,\text{pos}}||^2)}{(1+ \text{exp}(\Theta - ||\boldsymbol{y}_{i,\text{pos}}||^2))}\frac{\partial ||\boldsymbol{y}_{i,\text{pos}}||^2}{\partial W_1} + \frac{\text{exp}(||\boldsymbol{y}_{j,\text{neg}}||^2 - \Theta))}{(1+ \text{exp}(||\boldsymbol{y}_{j,\text{neg}}||^2 - \Theta)))}\frac{\partial ||\boldsymbol{y}_{j,\text{neg}}||^2}{\partial W_1}\\
    \frac{\partial \ell_{i,j}}{\partial W_2} &= \frac{-\text{exp}(\Theta - ||\boldsymbol{y}_{i,\text{pos}}||^2)}{(1+ \text{exp}(\Theta - ||\boldsymbol{y}_{i,\text{pos}}||^2))}\frac{\partial ||\boldsymbol{y}_{i,\text{pos}}||^2}{\partial W_2} + \frac{\text{exp}(||\boldsymbol{y}_{j,\text{neg}}||^2 - \Theta))}{(1+ \text{exp}(||\boldsymbol{y}_{j,\text{neg}}||^2 - \Theta)))}\frac{\partial ||\boldsymbol{y}_{j,\text{neg}}||^2}{\partial W_2}
\end{align}

As we consider that $f$ is a ReLU activation function such that $\frac{\partial ||\boldsymbol{y}_{i,\text{pos}}||^2}{\partial W_1} = \frac{\partial \boldsymbol{y}_{i,\text{pos}}^T\boldsymbol{y}_{i,\text{pos}}}{\partial W_1} = 2\cdot \text{diag}(f'_{\boldsymbol{y}_{i,\text{pos}}})\cdot \boldsymbol{y}_{i,\text{pos}} \cdot x_k^T$ where $\text{diag}(f'_{\boldsymbol{y}_{i,\text{pos}}})$ is a diagonal matrix with elements being the derivatives of ReLU applied element-wise to $\boldsymbol{y}_{i,\text{pos}}$. Therefore, we are able to obtain

\begin{align}
    \frac{\partial \ell_{i,j}}{\partial W_1} &= \frac{-\text{exp}(\Theta - ||\boldsymbol{y}_{i,\text{pos}}||^2)}{(1+ \text{exp}(\Theta - ||\boldsymbol{y}_{i,\text{pos}}||^2))}(2\cdot \text{diag}(f'_{\boldsymbol{y}_{i,\text{pos}}})\cdot \boldsymbol{y}_{i,\text{pos}} \cdot \boldsymbol{x}_k^T) + \nonumber\\&\frac{\text{exp}(||\boldsymbol{y}_{j,\text{neg}}||^2 - \Theta))}{(1+ \text{exp}(||\boldsymbol{y}_{j,\text{neg}}||^2 - \Theta)))}(2\cdot \text{diag}(f'_{\boldsymbol{y}_{j,\text{neg}}})\cdot \boldsymbol{y}_{j,\text{neg}} \cdot \boldsymbol{x}_k^T)\\
    \frac{\partial \ell_{i,j}}{\partial W_2} &= \frac{-\text{exp}(\Theta - ||\boldsymbol{y}_{i,\text{pos}}||^2)}{(1+ \text{exp}(\Theta - ||\boldsymbol{y}_{i,\text{pos}}||^2))}(2\cdot \text{diag}(f'_{\boldsymbol{y}_{i,\text{pos}}})\cdot \boldsymbol{y}_{i,\text{pos}} \cdot \boldsymbol{x}_k^T) + \nonumber\\
    &\frac{\text{exp}(||\boldsymbol{y}_{j,\text{neg}}||^2 - \Theta))}{(1+ \text{exp}(||\boldsymbol{y}_{j,\text{neg}}||^2 - \Theta)))}(2\cdot \text{diag}(f'_{\boldsymbol{y}_{j,\text{neg}}})\cdot \boldsymbol{y}_{j,\text{neg}} \cdot \boldsymbol{x}_n^T)
\end{align}

In each update for a batch of samples, we compute the average gradient of the Loss with respect to $W_1$ and $W_2$

\begin{align}
    \mathbb{E}_{i,j}[\frac{\partial \ell_{i,j}}{\partial W_1}] &= \mathbb{E}_{i}[\frac{-\text{exp}(\Theta - ||\boldsymbol{y}_{i,\text{pos}}||^2)}{(1+ \text{exp}(\Theta - ||\boldsymbol{y}_{i,\text{pos}}||^2))}(2\cdot \text{diag}(f'_{\boldsymbol{y}_{i,\text{pos}}})\cdot \boldsymbol{y}_{i,\text{pos}} \cdot \boldsymbol{x}_k^T)] + \nonumber\\&\mathbb{E}_{j}[\frac{\text{exp}(||\boldsymbol{y}_{j,\text{neg}}||^2 - \Theta))}{(1+ \text{exp}(||\boldsymbol{y}_{j,\text{neg}}||^2 - \Theta)))}(2\cdot \text{diag}(f'_{\boldsymbol{y}_{j,\text{neg}}})\cdot \boldsymbol{y}_{j,\text{neg}} \cdot \boldsymbol{x}_k^T)]\\
    \mathbb{E}_{i,j}[\frac{\partial \ell_{i,j}}{\partial W_2}] &= \mathbb{E}_{i}[\frac{-\text{exp}(\Theta - ||\boldsymbol{y}_{i,\text{pos}}||^2)}{(1+ \text{exp}(\Theta - ||\boldsymbol{y}_{i,\text{pos}}||^2))}(2\cdot \text{diag}(f'_{\boldsymbol{y}_{i,\text{pos}}})\cdot \boldsymbol{y}_{i,\text{pos}} \cdot \boldsymbol{x}_k^T)] + \nonumber\\&\mathbb{E}_{j}[\frac{\text{exp}(||\boldsymbol{y}_{j,\text{neg}}||^2 - \Theta))}{(1+ \text{exp}(||\boldsymbol{y}_{j,\text{neg}}||^2 - \Theta)))}(2\cdot \text{diag}(f'_{\boldsymbol{y}_{j,\text{neg}}})\cdot \boldsymbol{y}_{j,\text{neg}} \cdot \boldsymbol{x}_n^T)]
\end{align}

Practically, for each positive pair of $(\boldsymbol{x}_k, \boldsymbol{x}_k)$, pairs of $(\boldsymbol{x}_k, \boldsymbol{x}_n)$ and $(\boldsymbol{x}_n, \boldsymbol{x}_k)$ both work as negative samples. It is therefore natural to prove that

\begin{align}
\mathbb{E}_{j}\frac{\text{exp}(||\boldsymbol{y}_{j,\text{neg}}||^2 - \Theta))}{(1+ \text{exp}(||\boldsymbol{y}_{j,\text{neg}}||^2 - \Theta)))}(2\cdot \text{diag}(f'_{\boldsymbol{y}_{j,\text{neg}}})\cdot \boldsymbol{y}_{j,\text{neg}} \cdot \boldsymbol{x}_k^T) = \nonumber\\  \mathbb{E}_{j}\frac{\text{exp}(||\boldsymbol{y}_{j,\text{neg}}||^2 - \Theta))}{(1+ \text{exp}(||\boldsymbol{y}_{j,\text{neg}}||^2 - \Theta)))}(2\cdot \text{diag}(f'_{\boldsymbol{y}_{j,\text{neg}}})\cdot \boldsymbol{y}_{j,\text{neg}} \cdot \boldsymbol{x}_n^T)
\end{align}
Thus we have

\begin{align}
    \mathbb{E}_{i,j}[\frac{\partial L}{\partial W_1}] = \mathbb{E}_{i,j}[\frac{\partial L}{\partial W_2}]
\end{align}

The gradient of $W_1$ and $W_2$ goes into the same direction and thus converge to each other.

\newpage
\section{Theoretical analysis of distributions of positive and negative examples}\label{app-dis}

\begin{figure*}[ht]
%\vskip 0.2in
\begin{center}
\includegraphics[width=1\textwidth, clip=true, trim=2 2 2 2]{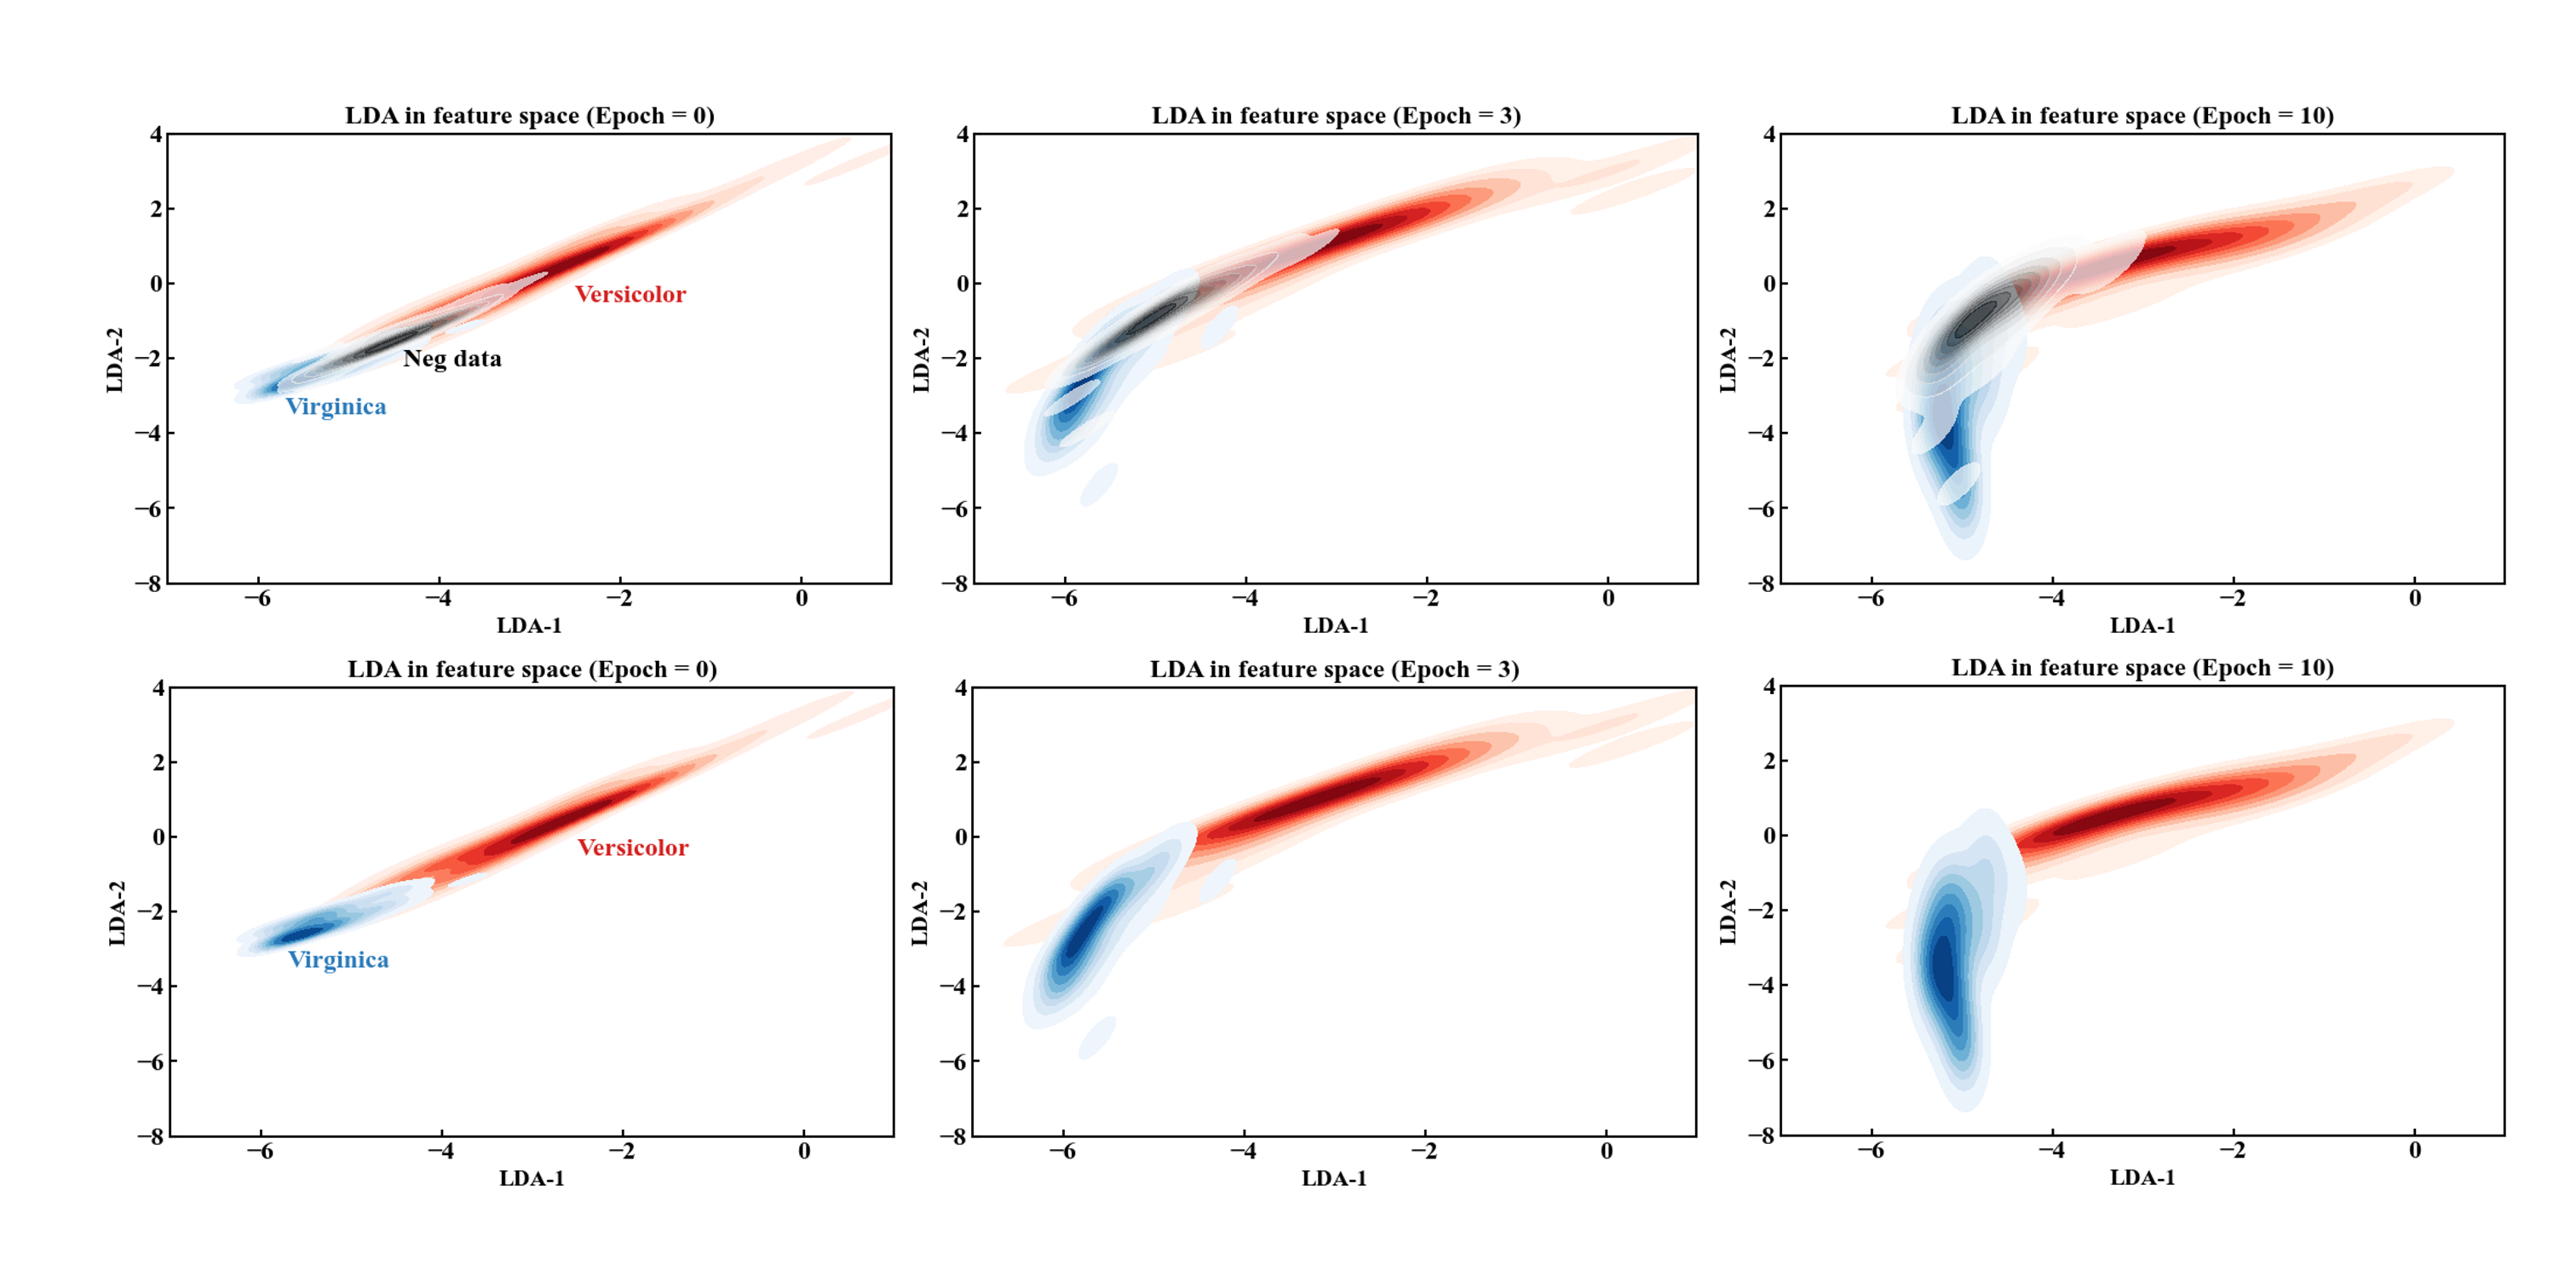}
\caption{Illustration of the evolution of feature separation in Linear Discriminant Analysis (LDA) space over different training epochs. The figures depict the separation between two positive examples (Versicolor and Virginica) in the feature space at different stages of training (Epoch 0, 3, and 10). Initially, at Epoch 0, the two positive examples exhibit significant overlap. As training progresses, the negative examples contribute to improving the separation between the positive examples. The negative examples provide contrast that aids in learning better decision boundaries, ultimately leading to more effective class separation. The first row includes also the position of negative examples during the train.}
\label{figs:lda_train}
\end{center}
%\vskip -0.2in
\end{figure*}

Assuming that each class of data samples follows a multivariate Gaussian distribution, which is a commonly used assumption \cite{S1}. Then, two examples $\boldsymbol{x}_{k}$ and  $\boldsymbol{x}_{n}$ taken from different classes would follow:
\begin{align*}
\boldsymbol{x}_{k} &\sim \mathcal{N}({\boldsymbol\mu}_1, \boldsymbol{\Sigma}_1) \\
\boldsymbol{x}_{n} &\sim \mathcal{N}(\boldsymbol{\mu}_2, \boldsymbol{\Sigma}_2)
\end{align*}
where \( \boldsymbol{\mu}_1 \) and \( \boldsymbol{\mu}_2 \) are the mean vectors of the two distributions, and \( \boldsymbol{\Sigma}_1 \) and \( \boldsymbol{\Sigma}_2 \) are their respective covariance matrices. Each class of distributions is assumed to be independent of each other.

Based on the previous conclusion that the input metrics $W_1$ and $W_2$ corresponding to the two concatenated images will converge to the same one and thus $W_1$ and $W_2$ is set to the same as $W = W_1 = W_2$ (the same case for all different network structures). The output becomes $\boldsymbol{y}_{i,\text{pos}}^{(0)} = f(2W\boldsymbol{x}_{k}$), $\boldsymbol{y}_{j,\text{neg}}^{(0)} = f(W(\boldsymbol{x}_{k} + \boldsymbol{x}_{n}))$. Thus, it is clealy seen that the positive and negative examples $\boldsymbol{x}_{i,\text{pos}}^{(0)}$, $\boldsymbol{x}_{j,\text{neg}}^{(0)}$ follow (considering $\boldsymbol{x}_{k}$ and $\boldsymbol{x}_{n}$ is independent of each other)
\begin{align*}
\boldsymbol{x}_{i,\text{pos}}^{(0)} \sim 2\boldsymbol{x}_{k} &\sim \mathcal{N}(2\boldsymbol{\mu}_1, 2\boldsymbol{\Sigma}_1) \\
\boldsymbol{x}_{j,\text{neg}}^{(0)} \sim \boldsymbol{x}_{k}+\boldsymbol{x}_{n}&\sim \mathcal{N}(\boldsymbol{\mu}_1+\boldsymbol{\mu}_2, \boldsymbol{\Sigma}_1+\boldsymbol{\Sigma}_2)
\end{align*}

By further assuming that all classes share the same covariance matrix \cite{S1}, i.e., $\boldsymbol{\Sigma}_1 = \boldsymbol{\Sigma}_2 = \boldsymbol{\Sigma}$, we have 
\begin{align*}
\boldsymbol{x}_{i,\text{pos}}^{(0)}&\sim \mathcal{N}(\boldsymbol{\mu}_{i,\text{p}}, \boldsymbol{\Sigma}_{i,\text{p}}) \sim \mathcal{N}(2\boldsymbol{\mu}_1, 2\boldsymbol{\Sigma}) \\
\boldsymbol{x}_{j,\text{neg}}^{(0)}&\sim \mathcal{N}(\boldsymbol{\mu}_{j,\text{n}}, \boldsymbol{\Sigma}_{j,\text{n}})\sim \mathcal{N}(\boldsymbol{\mu}_1+\boldsymbol{\mu}_2, 2\boldsymbol{\Sigma})
\end{align*}

It is immediately seen that the distributions of positive examples $\boldsymbol{x}_{i,\text{pos}}^{(0)}$ and negative examples $\boldsymbol{x}_{j,\text{neg}}^{(0)}$ share similar covariance properties. Besides, calculating Bhattacharya distance (or, similarly using KL divergence), which is a measure of divergence between two probability distributions, could give more intuitive understandings of the relative positions between two different positive examples or between positive and negative examples. Denoting $D_{pp}$ the distance between two positive distributions of 
$\boldsymbol{x}_{i,\text{pos}}^{(0)}$ and $\boldsymbol{x}_{j,\text{pos}}^{(0)}$, we have
\begin{align}
D_{pp} &= \frac{1}{8} (\boldsymbol{\mu}_{i,\text{p}} - \boldsymbol{\mu}_{j,\text{p}})^T \left( \frac{\boldsymbol{\Sigma}_{i,\text{p}} + \boldsymbol{\Sigma}_{j,\text{p}}}{2} \right)^{-1} (\boldsymbol{\mu}_{i,\text{p}} - \boldsymbol{\mu}_{j,\text{p}}) + \frac{1}{2} \log \left( \frac{\det \left( \frac{\boldsymbol{\Sigma}_{i,\text{p}} + \boldsymbol{\Sigma}_{j,\text{p}}}{2} \right)}{\sqrt{\det \boldsymbol{\Sigma}_{i,\text{p}} \cdot \det \boldsymbol{\Sigma}_{j,\text{p}}}} \right) \nonumber \\
& = \frac{1}{4} (\boldsymbol{\mu}_{1} - \boldsymbol{\mu}_{2})^T  \boldsymbol{\Sigma} ^{-1} (\boldsymbol{\mu}_{1} - \boldsymbol{\mu}_{2})
\end{align}

Similarly, the Bhattacharya distance $D_{pn}$ between two positive and negative distributions is calculated as
\begin{align}
D_{pn} &= \frac{1}{8} (\boldsymbol{\mu}_{i,\text{p}} - \boldsymbol{\mu}_{j,\text{n}})^T \left( \frac{\boldsymbol{\Sigma}_{i,\text{p}} + \boldsymbol{\Sigma}_{j,\text{n}}}{2} \right)^{-1} (\boldsymbol{\mu}_{i,\text{p}} - \boldsymbol{\mu}_{j,\text{n}}) + \frac{1}{2} \log \left( \frac{\det \left( \frac{\boldsymbol{\Sigma}_{i,\text{p}} + \boldsymbol{\Sigma}_{j,\text{n}}}{2} \right)}{\sqrt{\det \boldsymbol{\Sigma}_{i,\text{p}} \cdot \det \boldsymbol{\Sigma}_{j,\text{n}}}} \right) \nonumber \\
& = \frac{1}{16} (\boldsymbol{\mu}_{1} - \boldsymbol{\mu}_{2})^T  \boldsymbol{\Sigma} ^{-1} (\boldsymbol{\mu}_{1} - \boldsymbol{\mu}_{2})
\end{align}
Thus, we find that $D_{pn} = 1/4D_{pp}$. This indicates that the negative examples are consistently positioned between two distinct clusters of positive examples within the sample space.

When positive and negative examples are projected into the feature space through a neural network, the negative examples consistently play a crucial role in enhancing the separation between the positive examples. In Fig. \ref{figs:lda_train}, we demonstrate the progression of feature separation in Linear Discriminant Analysis (LDA) space across different training epochs using the Iris dataset, where the Versicolor and Virginica classes are inherently non-linearly separable. The features are first extracted via a single-layer neural network with 10 hidden neurons and subsequently mapped into the LDA space. At the initial stage (Epoch 0), there is significant overlap between the two positive classes. However, as training advances, the negative examples increasingly contribute to the improved separation of the positive classes by providing contrast that facilitates the learning of more distinct decision boundaries.

\section{
\color{blue}Mathematical Justification: Independent Layer Updates
}
\begingroup
\color{blue}

We demonstrate mathematically that weight updates in one layer do not affect the normalized input passed to the next layer, as shown in Hinton's work \cite{S5}. 
To see why, consider the FF update rule for neuron \( m \) in a given layer:

\begin{equation}
\Delta \boldsymbol{w}_m = 2\epsilon \frac{\partial \log(p)}{\partial \sum_m y_m^2} y_m \boldsymbol{x}^T
\end{equation}

where $p$ is either $p_{\text{pos}} = \sigma (\sum_m y_m^2 - \Theta)$ for a positive input or $p_{\text{neg}}  = \sigma (\Theta - \sum_m y_m^2)$ for a negative input. $\sigma$ is the sigmoid function and $\Theta$ is some threshold. \( \boldsymbol{w}_m \) is the weight vector for neuron \( m \). \( y_m \) is ReLU activation before layer normalization. \( \epsilon \) is the learning rate. \( \boldsymbol{x} \) is the input vector to the layer.

After applying the update, the new activation becomes:

\begin{equation}
y_m' = \boldsymbol{w}_m' \cdot \boldsymbol{x} = \left(\boldsymbol{w}_m + \Delta \boldsymbol{w}_m \right) \cdot \boldsymbol{x}
\end{equation}

Expanding the weight update:

\begin{equation}
y_m' = \boldsymbol{w}_m \cdot \boldsymbol{x} + 2\epsilon \frac{\partial \log(p)}{\partial \sum_m y_m^2} y_m (\boldsymbol{x}^T \cdot \boldsymbol{x})
\end{equation}

Since \( y_m = \boldsymbol{w}_m \cdot \boldsymbol{x} \), we obtain:

\begin{align}
y_m' &= y_m + 2\epsilon \frac{\partial \log(p)}{\partial \sum_m y_m^2} y_m ||\boldsymbol{x}||^2 \\
&= y_m \left(1 + 2\epsilon \frac{\partial \log(p)}{\partial \sum_m y_m^2} ||\boldsymbol{x}||^2 \right)
\end{align}

Define the scaling factor:

\begin{equation}
c = 1 + 2\epsilon \frac{\partial \log(p)}{\partial \sum_m y_m^2} ||\boldsymbol{x}||^2
\end{equation}

so that:

\begin{equation}
y_m' = c y_m
\end{equation}

Since all activations scale by the same factor \( c \), layer normalization (standardization which eliminates the mean and scales by the standard deviation of all activations in our case) cancels out this scaling, ensuring that the input to the next layer remains unchanged:

\begin{equation}
{\boldsymbol{y}}' = \frac{{c\boldsymbol{y}
}-c\mu}{c\cdot \text{std}(\boldsymbol{y})} = \frac{{\boldsymbol{y}
}-\mu}{\text{std}(\boldsymbol{y})}
\end{equation}
where $\boldsymbol{y}'$ and $\boldsymbol{y}$ are the vectors of output neurons after and before the update respectively, $\mu$ and $\text{std}(\boldsymbol{y})$ represent the mean and standard deviation of $\boldsymbol{y}$ respectively.
Thus, weight updates in previous layers do not affect the layer-normalized outputs, meaning that training layers independently does not introduce instability into subsequent layers. 

While mini-batch updates do not guarantee perfect proportional scaling as in the single-sample case, they generally approximate it well—especially when batch size is sufficiently large, ensuring statistical stability. Any small deviations in orientation are largely corrected by layer normalization, which ensures that the orientation of ${\boldsymbol{y}}'$ does not drastically change. 
This keeps each layer’s input to the next layer stable, ensuring that greedy layer-wise training and parallel, simultaneous updates yield similar results.
\endgroup

\newpage
\section{Detailed training algorithms}\label{app-alg}
We present the detailed algorithms for training with convolutional layers. Algorithm \ref{algorithm1-detail} describes the process of training a hidden layer using positive and negative examples directly derived from the output of the previous layer’s positive and negative examples. Algorithm \ref{algorithm2-detail} details the training process where positive and negative examples are generated by re-concatenating the previous layer's outputs to form new positive and negative examples. Differences between the two algorithms are highlighted in orange.%In practice, the first and the layer layers are trained with Algorithm \ref{algorithm1-detail} and the other hidden layers are trained with Algorithm \ref{algorithm2-detail}
\newline
\begin{algorithm}[H]
   \caption{SCFF's main learning algorithm 1}
   \label{algorithm1-detail}
\begin{algorithmic}

    %\Require $n \geq 0 \vee x \neq 0$
%\Ensure $y = x^n$
   \For{each layer of structure $f^{(l)}_\theta$, batch size $N$, threshold $\Theta_{\text{pos}}^{(l)}$,$\Theta_{\text{neg}}^{(l)}$}
   %\STATE {\bfseries Input:} batch size $N$, threshold $\Theta_{\text{pos}}^{l}$,$\Theta_{\text{neg}}^{l}$, penalized coefficient $\lambda^{l}$
   
    \For{sampled minibatch $\{\boldsymbol{x}_{k}\}_{k = 1}^{N}$}
   %\REPEAT
   \State randomly select an integer $s\in\{1, N\}$
%   \State for each $i\in\{1, N\}$ 
   \If{$l = 0$}
   \State \textcolor{gray}{\# form the positive and negative examples} 
   \State $\boldsymbol{x}_{k}$ = std($\boldsymbol{x}_{k}$)\hfill \textcolor{gray}{\# standardization} 
   \State$\boldsymbol{x}_{i,\text{pos}}^{(l)}$ = cat([$\boldsymbol{x}_{k}, \boldsymbol{x}_{k}$], dim = 1) \hfill \textcolor{gray}{\# concatenation} 
   \State$\boldsymbol{x}_{j,\text{neg}}^{(l)}$ = cat([$\boldsymbol{x}_{k}, \boldsymbol{x}_{n}$], dim = 1) where $n = (k+s)\%N$ 
    \Else 
    \State \textcolor{gray}{\# for $l>0$} 
    \State\textcolor{orange}{$\boldsymbol{x}_{i,\text{pos}}^{(l)}$ = $\boldsymbol{y}_{i,\text{pos}}^{(l-1)}$\hfill \textcolor{gray}{\# previous layer output} 
   \State$\boldsymbol{x}_{j,\text{neg}}^{(l)}$ = $\boldsymbol{y}_{j,\text{neg}}^{(l-1)}$ }
   %\vspace{\baselineskip}
    \EndIf
   %\vspace{\baselineskip}\\
   \State $\boldsymbol{x}_{i,\text{pos}}^{(l)}$ = std($\boldsymbol{x}_{i,\text{pos}}^{(l)}$); $\boldsymbol{x}_{j,\text{neg}}^{(l)}$ = std($\boldsymbol{x}_{j,\text{neg}}^{(l)}$)\hfill \textcolor{gray}{\# standardization} 
   %\State$\boldsymbol{x}_{j,\text{neg}}^{(l)}$ = std($\boldsymbol{x}_{j,\text{neg}}^{(l)}$) 
   %\vspace{\baselineskip}
   \State $\boldsymbol{y}_{i,\text{pos}}^{(l)} = f^{(l)}_\theta(\boldsymbol{x}_{i,\text{pos}})$; $\boldsymbol{y}_{j,\text{neg}}^{(l)} = f^{(l)}_\theta(\boldsymbol{x}_{j,\text{neg}})$ \hfill \textcolor{gray}{\# output [C, H, W]} 
    %\State$\boldsymbol{y}_{j,\text{neg}}^{(l)} = f^{(l)}_\theta(\boldsymbol{x}_{j,\text{neg}})$
    %\vspace{\baselineskip}
    \State \textcolor{gray}{\# calculate the goodness} 
    \State$G_{i,\text{pos}}^{(l)} = \frac{1}{C}\sum_c{y_{i,c,h, w,\text{pos}}^{2(l)}}$; $G_{j,\text{neg}}^{(l)} = \frac{1}{C}\sum_c{y_{j,c,h, w,\text{neg}}^{2(l)}}$ \hfill \textcolor{gray}{\# output [H, W]}
    %\State$G_{j,\text{neg}}^{(l)} = \frac{1}{C}\sum_c{y_{j,c,h, w,\text{neg}}^{2(l)}}$\\  
    %\vspace{\baselineskip}
    %\State \textcolor{gray}{\# $\ell(\theta)$ to maximize/minimize goodness for positive/negative examples} 
    \State \textcolor{gray}{\# $\mathcal{L}_{\text{SCFF}}^{(l)}$ is initialized as 0 at each layer and is accumulated for each batch}
    \State$\mathcal{L}_{\text{SCFF}}^{(l)} =\mathcal{L}_{\text{SCFF}}^{(l)} +\ell_{i,j}$
    %\State$\mathcal{L} = %\mathcal{L}_\text{CFF} + \lambda^{l}||G_{i,\text{pos}}^{(l)}||_F $
    %\State update network $f^{l}$ to minimize $\mathcal{L}$\\
    %\\
    \State \textcolor{gray}{\# triangle method to transmit previous layer's information} 
    \State$\boldsymbol{y}_{i,\text{pos}}^{(l)}$ = triangle($\boldsymbol{y}_{i,\text{pos}}^{(l)}$); $\boldsymbol{y}_{j,\text{neg}}^{(l)}$ = triangle($\boldsymbol{y}_{j,\text{neg}}^{(l)}$)
    %\State$\boldsymbol{y}_{j,\text{neg}}^{(l)}$ = triangle($\boldsymbol{y}_{j,\text{neg}}^{(l)}$)  \hfill %\textcolor{gray}{\# triangle method to transmit previous layer information} \\
   \EndFor
   \State Use optimizer to update network $f^{(l)}_\theta$ to minimize $\mathcal{L}_{\text{SCFF}}^{(l)}$
   %\\
    \State \textcolor{gray}{\# pooling operation to reduces the size of the feature maps} \State$\boldsymbol{y}_{i,\text{pos}}^{(l)}$ = POOL($\boldsymbol{y}_{i,\text{pos}}^{(l)}$); $\boldsymbol{y}_{j,\text{neg}}^{(l)}$ = POOL($\boldsymbol{y}_{j,\text{neg}}^{(l)}$)
   %\State$\boldsymbol{y}_{j,\text{neg}}^{(l)}$ = POOL($\boldsymbol{y}_{j,\text{neg}}^{(l)}$) 

   \EndFor

   %\UNTIL{$noChange$ is $true$}
\end{algorithmic}
\end{algorithm}

\begin{algorithm}[H]
   \caption{SCFF's main learning algorithm 2}
   \label{algorithm2-detail}
\begin{algorithmic}
    %\Require $n \geq 0 \vee x \neq 0$
    %\Ensure $y = x^n$
   \For{each layer of structure $f^{(l)}_\theta$, batch size $N$, threshold $\Theta_{\text{pos}}^{(l)}$,$\Theta_{\text{neg}}^{(l)}$}
   %\STATE {\bfseries Input:} batch size $N$, threshold $\Theta_{\text{pos}}^{l}$,$\Theta_{\text{neg}}^{l}$, penalized coefficient $\lambda^{l}$
   
    \For{sampled minibatch $\{\boldsymbol{x}_{k}\}_{k = 1}^{N}$}
   %\REPEAT
   \State randomly select an integer $s\in\{1, N\}$
   %\State for each $i\in\{1, N\}$ \\
   \If{$l = 0$}
   \State \textcolor{gray}{\# form the positive and negative examples} 
   \State $\boldsymbol{x}_{k}$ = std($\boldsymbol{x}_{k}$)\hfill \textcolor{gray}{\# standardization} 
   \State$\boldsymbol{x}_{i,\text{pos}}^{(l)}$ = cat([$\boldsymbol{x}_{k}, \boldsymbol{x}_{k}$], dim = 1) \hfill \textcolor{gray}{\# concatenation} 
   \State$\boldsymbol{x}_{j,\text{neg}}^{(l)}$ = cat([$\boldsymbol{x}_{k}, \boldsymbol{x}_{n}$], dim = 1) where $n = (k+s)\%N$ 
    \Else 
    \State \textcolor{gray}{\# for $l>0$} 
    \State \textcolor{gray}{\# reconcatenation to form new positive and negative examples} 
    \State\textcolor{orange}{$\boldsymbol{x}_{i,\text{pos}}^{(l)}$ = cat([std($\boldsymbol{y}_{i,\text{pos}}^{(l-1)}$), std($\boldsymbol{y}_{i,\text{pos}}^{(l-1)}$)], dim = 1) 
   \State$\boldsymbol{x}_{i,\text{neg}}^{(l)}$ = cat([std($\boldsymbol{y}_{j,\text{pos}}^{(l-1)}$), std($\boldsymbol{y}_{j,\text{pos}}^{(l-1)}$)], dim = 1) where $j = (k+s)\%N$}
   %\vspace{\baselineskip}
    \EndIf
   %\vspace{\baselineskip}\\
   \State $\boldsymbol{x}_{i,\text{pos}}^{(l)}$ = std($\boldsymbol{x}_{i,\text{pos}}^{(l)}$); $\boldsymbol{x}_{j,\text{neg}}^{(l)}$ = std($\boldsymbol{x}_{j,\text{neg}}^{(l)}$)\hfill \textcolor{gray}{\# standardization} 
   %\State$\boldsymbol{x}_{j,\text{neg}}^{(l)}$ = std($\boldsymbol{x}_{j,\text{neg}}^{(l)}$) 
   %\vspace{\baselineskip}
   \State $\boldsymbol{y}_{i,\text{pos}}^{(l)} = f^{(l)}_\theta(\boldsymbol{x}_{i,\text{pos}})$; $\boldsymbol{y}_{j,\text{neg}}^{(l)} = f^{(l)}_\theta(\boldsymbol{x}_{j,\text{neg}})$ \hfill \textcolor{gray}{\# output [C, H, W]}
    %\State$\boldsymbol{y}_{j,\text{neg}}^{(l)} = f^{(l)}_\theta(\boldsymbol{x}_{j,\text{neg}})$\\
    %\vspace{\baselineskip}\\
    \State \textcolor{gray}{\# calculate the goodness} 
    \State$G_{i,\text{pos}}^{(l)} = \frac{1}{C}\sum_c{y_{i,c,h, w,\text{pos}}^{2(l)}}$; $G_{j,\text{neg}}^{(l)} = \frac{1}{C}\sum_c{y_{j,c,h, w,\text{neg}}^{2(l)}}$ \hfill \textcolor{gray}{\# output [H, W]}
    %\State$G_{j,\text{neg}}^{(l)} = \frac{1}{C}\sum_c{y_{j,c,h, w,\text{neg}}^{2(l)}}$\\  
    %\vspace{\baselineskip}\
    \State \textcolor{gray}{\# $\mathcal{L}_{\text{SCFF}}^{(l)}$ is initialized as 0 at each layer and is accumulated for each batch}
    \State$\mathcal{L}_{\text{SCFF}}^{(l)} =\mathcal{L}_{\text{SCFF}}^{(l)} +\ell_{i,j}$
    %\State$\mathcal{L} = %\mathcal{L}_\text{CFF} + \lambda^{l}||G_{i,\text{pos}}^{(l)}||_F $
    %\State update network $f^{l}$ to minimize $\mathcal{L}$\\
    %\\
    \State \textcolor{gray}{\# triangle method to transmit previous layer information to the next layer} 
    \State$\boldsymbol{y}_{i,\text{pos}}^{(l)}$ = triangle($\boldsymbol{y}_{i,\text{pos}}^{(l)}$); $\boldsymbol{y}_{j,\text{neg}}^{(l)}$ = triangle($\boldsymbol{y}_{j,\text{neg}}^{(l)}$)
    %\State$\boldsymbol{y}_{j,\text{neg}}^{(l)}$ = triangle($\boldsymbol{y}_{j,\text{neg}}^{(l)}$)  \hfill %\textcolor{gray}{\# triangle method to transmit previous layer information} \\
   \EndFor
   \State Use optimizer to update network $f^{(l)}_\theta$ to minimize $\mathcal{L}_{\text{SCFF}}^{(l)}$
\State \textcolor{gray}{\# pooling operation to reduces the size of the feature maps} \State$\boldsymbol{y}_{i,\text{pos}}^{(l)}$ = POOL($\boldsymbol{y}_{i,\text{pos}}^{(l)}$); $\boldsymbol{y}_{j,\text{neg}}^{(l)}$ = POOL($\boldsymbol{y}_{j,\text{neg}}^{(l)}$)

   \EndFor

   %\UNTIL{$noChange$ is $true$}
\end{algorithmic}
\end{algorithm}

\newpage
\section{Convolutional Layer architecture}
\label{app-cnnarc}
In each layer, the input data is first processed by a convolutional layer, followed by either a "triangle" activation function or a ReLU activation, and then a pooling operation (as shown in the "CIFAR-10", "STL-10" \textcolor{blue}{and "Tiny ImageNet"} columns of Table \ref{tab:arch}). It's important to note that the activations listed in Table \ref{tab:arch} are used solely for passing information to the next layer, whereas the activation function used for plasticity, i.e., during training, is consistently set as ReLU throughout all layers. \textcolor{blue}{}{For the CIFAR-10 and STL-10 datasets}, the first layer had a width of 96 convolutional kernels, as described in \cite{S2}. The number of kernels in subsequent layers was scaled by a factor of 4 relative to the previous layer. \textcolor{blue}{For the Tiny ImageNet dataset, we use an AlexNet-like architecture with a filter size configuration of 64-192-384-256-256.}

To assess the performance of each layer, hidden neuronal activities are extracted from the pooling layer using an additional pooling operation (as shown in the "Layer's output" column of Table \ref{tab:arch}) with the stride size matching the kernel size to reduce dimensionality. For the CIFAR-10 dataset, the final accuracy is calculated by aggregating the output neurons from all layers and using them as input to a linear classifier. For the STL-10 dataset, the final accuracy is derived by combining the output neurons from the last two layers (Layer 3 and Layer 4) and feeding them into a linear classifier. \textcolor{blue}{For the Tiny ImageNet dataset, the final accuracy is determined by combining the output neurons from all layers except the first layer and passing them into a linear classifier.} Other detailed architecture parameters are listed in the Table \ref{tab:arch}. 

\begin{table}[ht]
\centering
\tiny
\caption{Layer configurations across different datasets. The CIFAR-10 and STL-10 columns detail the structure of each layer, corresponding to the layer numbers listed in the first column. The "Layer's Output" column presents the additional pooling operation from the corresponding pooling layer, as indicated by the blue arrows, to form the input for the final linear classifier.} % Add your table caption here

\begin{tabular}{cccccccccc}

\toprule
{\makecell{{\#} \\{layer}} } & {CIFAR-10} & {} &{\makecell{{Layer's} \\{output} }} & {STL-10} &{} &{\makecell{{Layer's} \\{output} }}  & \textcolor{blue}{\makecell{{Tiny} \\{ImageNet} }  } &{} &{\makecell{\textcolor{blue}{Layer's} \\\textcolor{blue}{output} }}\\
\midrule
1 & \begin{tabular}[c]{@{}c@{}}5x5 Conv96\footnotemark[1]\\ Triangle\\ 4x4 MaxPool\footnotemark[3]\end{tabular} & \begin{tabular}[c]{@{}c@{}} {}\\ {}\\$\textcolor{blue}{\rightarrow}$\end{tabular}& \begin{tabular}[c]{@{}c@{}} {}\\ {}\\ 2x2 AvgPool\footnotemark[5]\end{tabular} & \begin{tabular}[c]{@{}c@{}} 5x5 Conv96\footnotemark[1]\\ Triangle\\ 4x4 MaxPool\footnotemark[3]\end{tabular} & \begin{tabular}[c]{@{}c@{}} {}\\ {}\\$\textcolor{blue}{\rightarrow}$\end{tabular} & \begin{tabular}[c]{@{}c@{}} {}\\ {}\\ 4x4 AvgPool\footnotemark[5]\end{tabular}& \textcolor{blue}{\begin{tabular}[c]{@{}c@{}}5x5 Conv64\footnotemark[1]\\ Triangle\\ 2x2 MaxPool\footnotemark[4]\end{tabular}} & \begin{tabular}[c]{@{}c@{}} {}\\ {}\\ {}\end{tabular} & \textcolor{blue}{\begin{tabular}[c]{@{}c@{}} {}\\ {}\\ {}\end{tabular}} \\ 
\midrule 
2 & \begin{tabular}[c]{@{}c@{}} 3x3 Conv384\footnotemark[2]\\ Triangle\\ 4x4 MaxPool\footnotemark[3]\end{tabular} & \begin{tabular}[c]{@{}c@{}} {}\\ {}\\$\textcolor{blue}{\rightarrow}$ \end{tabular} & \begin{tabular}[c]{@{}c@{}} {}\\ {}\\ {2x2 AvgPool\footnotemark[5]}\end{tabular}& \begin{tabular}[c]{@{}c@{}} 3x3 Conv384\footnotemark[2]\\ Triangle\\ 4x4 MaxPool\footnotemark[3]\end{tabular} & \begin{tabular}[c]{@{}c@{}} {}\\ {}\\$\textcolor{blue}{\rightarrow}$\end{tabular} & \begin{tabular}[c]{@{}c@{}} {}\\ {}\\ 4x4 AvgPool\footnotemark[5]\end{tabular} & \textcolor{blue}{\begin{tabular}[c]{@{}c@{}} 3x3 Conv192\footnotemark[2]\\ Triangle\\ 2x2 MaxPool\footnotemark[4]\end{tabular}} & \begin{tabular}[c]{@{}c@{}} {}\\ {}\\$\textcolor{blue}{\rightarrow}$\end{tabular} & \begin{tabular}[c]{@{}c@{}} {}\\ {}\\ \textcolor{blue}{4x4 AvgPool\footnotemark[5]}\end{tabular} \\
\midrule
3 & \begin{tabular}[c]{@{}c@{}} 3x3 Conv1536\footnotemark[2]\\ {ReLU}\\ {2x2 AvgPool\footnotemark[4]}\end{tabular} & \begin{tabular}[c]{@{}c@{}} {}\\ {}\\ {$\textcolor{blue}{\rightarrow}$}\end{tabular} & \begin{tabular}[c]{@{}c@{}} {}\\ {}\\ 2x2 AvgPool\footnotemark[5]\end{tabular} & \begin{tabular}[c]{@{}c@{}} 3x3 Conv1536\footnotemark[2]\\ {ReLU}\\ 4x4 {}MaxPool\footnotemark[3]\end{tabular} & \begin{tabular}[c]{@{}c@{}} {}\\ {}\\{$\textcolor{blue}{\rightarrow}$}\end{tabular} & \begin{tabular}[c]{@{}c@{}} {}\\ {}\\ 4x4 AvgPool\footnotemark[5]\end{tabular}& \textcolor{blue}{\begin{tabular}[c]{@{}c@{}} 3x3 Conv384\footnotemark[2]\\ Triangle\\ 1x1 MaxPool\footnotemark[6]\end{tabular}} & \begin{tabular}[c]{@{}c@{}} {}\\ {}\\$\textcolor{blue}{\rightarrow}$\end{tabular} & \begin{tabular}[c]{@{}c@{}} {}\\ {}\\ \textcolor{blue}{4x4 AvgPool\footnotemark[5]}\end{tabular}\\
\midrule
4 & & \begin{tabular}[c]{@{}c@{}} {}\\ {}\\ {}\end{tabular} & \begin{tabular}[c]{@{}c@{}} {}\\ {}\\ {}\end{tabular} & \begin{tabular}[c]{@{}c@{}} 3x3 Conv6144\footnotemark[2]\\ {Triangle}\\ {2x2 MaxPool\footnotemark[4]}\end{tabular}& \begin{tabular}[c]{@{}c@{}} {}\\ {}\\{$\textcolor{blue}{\rightarrow}$}\end{tabular} & \begin{tabular}[c]{@{}c@{}} {}\\ {}\\ 3x3 MaxPool\footnotemark[5]\end{tabular}& \textcolor{blue}{\begin{tabular}[c]{@{}c@{}} 3x3 Conv256\footnotemark[2]\\ Triangle\\ 1x1 MaxPool\footnotemark[6]\end{tabular}} & \begin{tabular}[c]{@{}c@{}} {}\\ {}\\$\textcolor{blue}{\rightarrow}$\end{tabular} & \begin{tabular}[c]{@{}c@{}} {}\\ {}\\ \textcolor{blue}{4x4 AvgPool\footnotemark[5]}\end{tabular}
\\
\midrule
5 & & & & & & & \textcolor{blue}{\begin{tabular}[c]{@{}c@{}} 3x3 Conv256\footnotemark[2]\\ ReLU\\ 2x2 MaxPool\footnotemark[4]\end{tabular}} & \begin{tabular}[c]{@{}c@{}} {}\\ {}\\$\textcolor{blue}{\rightarrow}$\end{tabular} & \begin{tabular}[c]{@{}c@{}} {}\\ {}\\ \textcolor{blue}{4x4 AvgPool\footnotemark[5]}\end{tabular}
\\

\bottomrule
\end{tabular}
\footnotetext[1]{With pad size of 2 and stride size of 1}
\footnotetext[2]{With pad size of 1 and stride size of 1}
\footnotetext[3]{With pad size of 1 and stride size of 2}
\footnotetext[4]{With pad size of 0 and stride size of 2}
\footnotetext[5]{With pad size of 0 and stride size the same as kernel size}
{\footnotetext[6]{\textcolor{blue}{With pad size of 0 and stride size of 1}}}

\label{tab:arch}
\end{table}

\newpage
\section{Recurrent Layer architecture}
\label{app-rnn}
The bi-directional recurrent layer comprises two RNNs that process the sequence in opposite directions: one from the start to the end, and the other from the end to the start. Each RNN is composed of 500 hidden neurons. The input Mel-frequency Cepstral Coefficients (MFCC) feature at each time step is standardized before being fed into the hidden neurons. Additionally, the output hidden state at each time step is standardized before being passed to the next time step as the preceding state. The final output is generated by merging the outputs from the last time step of each direction, which is then used as input to the final linear classifier. 

The MFCC features are derived from the audio waveform through a series of transformations that convert the raw audio signal into a representation that captures the phonetic content of speech, making it ideal for tasks like speech recognition. In our experiment, the audio is sampled at 16,000 Hz, and 39 MFCC coefficients are extracted.

\newpage
\section{Hyperparameter optimization}
\label{app-hyper}
We conducted a systematic investigation to determine the optimal set of hyperparameters for each hidden layer across all datasets.

We reserved a portion of the training set for validation purposes during hyperparameter tuning (20\% for CIFAR-10 and STL-10, 10\% for FSDD, and 10,000 samples from the MNIST dataset). Once the optimal hyperparameters were identified on the validation set, we retrained the model using the entire training and validation sets combined. The final test accuracy was then reported. \textcolor{blue}{For Tiny ImageNet, we report validation accuracy on its 10,000 images as the final result, since test labels are unavailable.}

The classifier used in our experiments is a simple linear model trained directly on the outputs of the hidden layers (refer to Appendix \ref{app-cnnarc} for details on retrieving the layer outputs and refer to Appendix \ref{app-lindout} for the linear evaluation). 

For data augmentation, we applied specific techniques based on the dataset: random horizontal flip for CIFAR-10, and padding followed by random cropping and horizontal flipping for STL-10 \textcolor{blue}{and Tiny ImageNet}. 
\begin{lstlisting}
# CIFAR-10:
transform = transforms.Compose([
    transforms.RandomHorizontalFlip(),
    transforms.ToTensor(),
    transforms.Normalize((0.4914, 0.4822, 0.4465), (0.2023, 0.1994, 0.2010)),
])
\end{lstlisting}
\begin{lstlisting}
# STL-10:
transform = transforms.Compose([
    transforms.RandomCrop(96, padding=4),
    transforms.RandomHorizontalFlip(),
    transforms.ToTensor(),
    transforms.Normalize((0.4914, 0.4822, 0.4465), (0.2471, 0.2435, 0.2616)),
])
\end{lstlisting}
\begin{lstlisting}
# Tiny ImageNet:
transform = transforms.Compose([
    transforms.RandomCrop(64, padding=2),
    transforms.RandomHorizontalFlip(),
    transforms.ToTensor(),
    transforms.Normalize((0.4914, 0.4822, 0.4465), (0.2471, 0.2435, 0.2616)),
])
\end{lstlisting}

The networks were trained using the Adam optimizer with weight decay, along with an Exponential Learning Rate Scheduler. To search for the best hyperparameters, we utilized Optuna \cite{S3}. 

\textcolor{blue}{For greedy layer-wise training, each layer of the network is fully trained before proceeding to the next layer. In joint training, all layers are updated simultaneously using SCFF’s local learning rule in each iteration.}

\subsection{\textcolor{blue}{Greedy layer-wise training}}

\textcolor{blue}{The architectures used for training on CIFAR-10 and STL-10 are provided in Appendix \ref{app-cnnarc}, while the architecture for training on FSDD is detailed in Appendix \ref{app-rnn}. For the MNIST dataset, we use a two-layer MLP, with each layer containing 2000 hidden neurons. We used a batch size of 100 for the MNIST, CIFAR-10, and STL-10 datasets, and a batch size of 64 for the FSDD dataset.} The complete set of hyperparameters 
\textcolor{blue}{for greedy layer-wise training} is detailed in Tables \ref{tab:hypermnist}, \ref{tab:hypercifar}, \ref{tab:hyperstl} and \ref{tab:hyperpars2}, \textcolor{blue}{corresponding to the  CIFAR-10, MNIST, STL-10, and FSDD datasets, respectively. The definition of those hyper-parameters are defined in Table \ref{tab:hypercifar}.}

\begin{comment}
    \begin{table}[ht]
\centering
\caption{Best hyper-parameters searched for CIFAR-10 and STL-10 datasets.}
\begin{tabular}{lcccccccccccccc}
\toprule
Layer & \multicolumn{7}{c}{CIFAR-10} & \multicolumn{7}{c}{STL-10}\\
\cmidrule(lr){2-8} \cmidrule(lr){9-15}
        & $lr$ & $\Theta_{\text{pos}}$ & $\Theta_{\text{neg}}$ & $\lambda$ & $w_d$ & $\gamma$ & $\text{al}$ & $lr$ & $\Theta_{\text{pos}}$ & $\Theta_{\text{neg}}$ & $\lambda$ & $w_d$ & $\gamma$ & $\text{al}$ \\
\midrule
1     & 0.01     & 0     & 1    & 1e-3    &  0.026     & 0     & 2    & 0 \\
2 & 0.002     & 5     & 9    & 7e-4      &0.003     & 8     & 10    & 0.0015 \\
3 & 0.0002     & 6     & 10    & 5e-4      &0.001     & 9     & 6    & 0.005 \\
4 & {}     & {}     & {}    & {}      &0.0001     & 6     & 9    & 0.005 \\
\bottomrule
\end{tabular}

\label{tab:hyperpars1}
\end{table}
\end{comment}

\begin{table*}[ht]
\centering
\caption{Hyper-parameters for \textcolor{blue}{greedy layer-wise training on} CIFAR-10 dataset.}
\begin{threeparttable}
\begin{tabular}{lccccccccc}
\toprule
Layer %& \multicolumn{9}{c}{CIFAR-10} \\
%\cmidrule(lr){2-10} 
        & $lr$\footnotemark[1] & $\Theta_{\text{pos}}$ & $\Theta_{\text{neg}}$ & $\lambda$ & $w_d$\footnotemark[2] & $\gamma$\footnotemark[3] & $\text{Alg}$\footnotemark[4] & $\text{Dropout}$\footnotemark[5] & $\text{Epochs}$\footnotemark[6]\\
\midrule
1     & 0.01     & 0     & 1    & 0    & 0.0001 & 0.7 & {$\/$} & 0.1 & 10\\
2 & 0.002     & 5     & 9    & 0.0007    & 0.0001 & 0.8 & "1" & 0.1  & 10 \\
3 & 0.0002     & 6     & 10    & 0.0005 & 0.0003 & 1 & "2" & 0.2  & 25  \\
\bottomrule
\end{tabular}
\begin{tablenotes}
\footnotesize
\item[1] $w_d$: Learning rate of the AdamW optimizer.
\item[2] $w_d$: Weight decay coefficient of the AdamW optimizer.
\item[3] $\gamma$: Multiplicative factor of learning rate decay (Exponential LR scheduler).
\item[4] $\text{Alg}$: "1" represents Algorithm 1 and "2" represents Algorithm 2 in Appendix \ref{app-alg}.
\item[5] $\text{Dropout}$: Dropout rate of the linear classifer.
\item[6] $\text{Epochs}$: Maximum epochs needed to train.
\end{tablenotes}
\end{threeparttable}

\label{tab:hypercifar}
\end{table*}

\begin{table*}[ht]
\centering
\caption{Hyper-parameters for \textcolor{blue}{greedy layer-wise training on} MNIST \textcolor{blue}{(MLP)} dataset.}
\begin{tabular}{lcccccccc}
\toprule
Layer  %& \multicolumn{8}{c}{MNIST}\\
%\cmidrule(lr){2-9} 
        & $lr$ & $\Theta_{\text{pos}}$ & $\Theta_{\text{neg}}$ & $\lambda$ & $w_d$ & $\gamma$ & $\text{Dropout}$ & $\text{Epochs}$ \\
\midrule
1   &  0.003     & 4     & 6    & 0.0001 & 1e-5 & 0.9  & 0.1  & 20\\
2   &0.002     & 1     & 1    & 0 & {1e-5} & {0.6} & 0.2  & 20 \\
\bottomrule
\end{tabular}
\label{tab:hypermnist}
\end{table*}

\begin{table*}[ht]
\centering
\caption{Hyper-parameters for \textcolor{blue}{greedy layer-wise training on} STL-10 dataset.}
\begin{tabular}{lccccccccc}
\toprule
Layer  %& \multicolumn{9}{c}{STL-10}\\
%\cmidrule(lr){2-10} 
        & $lr$ & $\Theta_{\text{pos}}$ & $\Theta_{\text{neg}}$ & $\lambda$ & $w_d$ & $\gamma$ & $\text{Alg}$ & $\text{Dropout}$ & $\text{Epochs}$ \\
\midrule
1   &  0.026     & 0     & 2    & 0 & 0.001 & 0.99 & {} & 0.4  & 8\\
2   &0.003     & 5     & 8    & 0.0015 & {0.0003} & {0.8} & "1" & 0.4  & 10 \\
3   &0.001     & 6     & 8    & 0.005 & 0 & 0.99 & "1" & 0.4  & 10\\
4   &0.0001     & 5     & 10    & 0.006 & 0.001 & 1 & "2" & 0.6 & 30\\
\bottomrule
\end{tabular}
\label{tab:hyperstl}
\end{table*}

\begin{table*}[ht]
\centering
\caption{Hyper-parameters for FSDD datasets.}
\begin{tabular}{lcccccccc}
\toprule
Layer %& \multicolumn{4}{c}{MNIST} & \multicolumn{4}{c}{FSDD}\\
%\cmidrule(lr){2-5} \cmidrule(lr){6-9}
        & $lr$ & $\Theta_{\text{pos}}$ & $\Theta_{\text{neg}}$ & $\lambda$ & $w_d$ & $\gamma$ & $\text{Dropout}$ & $\text{Epochs}$ \\
\midrule
1     & 2e-5     & 0     & 1    & 0.0075    &  0     & 0.7     & 0    & 10 \\
\bottomrule
\end{tabular}
\label{tab:hyperpars2}
\end{table*}

\subsubsection{Impact of $\lambda$, $\Theta_{\text{pos}}$ and $\Theta_{\text{neg}}$ on learning performance}

The choice of hyperparameters such as $\lambda$, $\Theta_{\text{pos}}$, and $\Theta_{\text{neg}}$ significantly impacts the learning performance. Table \ref{tab:eval_lamda} presents the test accuracies on the CIFAR-10 dataset when the penalty term is either included ($\lambda^{(2)} = 5e-4$) or excluded ($\lambda^{(2)} = 0$) from the training loss, for various threshold values of $\Theta_{\text{pos}}$ during the training of the third convolutional layer. The results demonstrate that incorporating the penalty term consistently enhances training performance compared to omitting it.

Table \ref{tab:eval_theta} further explores the test accuracies for different combinations of threshold values for $\Theta_{\text{pos}}^{(2)}$ and $\Theta_{\text{neg}}^{(2)}$ on the CIFAR-10 dataset. The results indicate that the highest accuracy is achieved when $\Theta_{\text{pos}}^{(2)}$ is slightly smaller than $\Theta_{\text{neg}}^{(2)}$.

Across all experiments, the optimal accuracy is typically reached within 25 epochs, with each reported accuracy representing the average of three runs using different random seeds.

\begin{table*}[ht]
\centering
\caption{Test accuracy (\%) vs $\lambda^{(2)}$ for different $\Theta_{\text{pos}}^{(2)}$ on CIFAR-10 dataset. $\Theta_{\text{neg}}^{(2)} = 10$.}
\begin{tabular}{lcccccc}
\toprule

{$\Theta_{\text{pos}}^{(2)}$} & {5} & {6} & {7} & {8} & {9} \\
\midrule
$\lambda^{(2)} = 0$ & 80.50 & 80.58 & 80.55 & 80.40 & 80.44\\
$\lambda^{(2)} = 5e-4$ & \textbf{80.70} & \textbf{80.75} & \textbf{80.64} & \textbf{80.57} & \textbf{80.54}\\
\bottomrule
\end{tabular}
\label{tab:eval_lamda}
\end{table*}

\begin{table*}[ht]
\centering
\caption{Test accuracy (\%) vs $\Theta_{\text{pos}}^{(2)}$ and  $\Theta_{\text{neg}}^{(2)}$ on CIFAR-10 dataset. $\lambda^{(2)} = 5e-4$.}
\begin{tabular}{lcccccccccc}
\toprule
$\Theta_{\text{pos}}^{(2)}$ & {1} & {2} & {3}& {4}& {5}& {6}& {7}& {8} & {9}\\
\midrule
$\Theta_{\text{neg}}^{(2)} = 9$ & 80.61 & 80.55 & 80.65 & 80.64 & 80.62 & 80.64 & 80.63 & 80.46 & 80.44 \\
$\Theta_{\text{neg}}^{(2)} = 10$ & 80.46 & 80.48 & 80.50 & 80.63 & 80.70 & \textbf{80.75} & 80.64 & 80.57 & 80.54\\
\bottomrule
\end{tabular}
\label{tab:eval_theta}
\end{table*}

\subsection{\textcolor{blue}{Joint training}}
\begingroup
\color{blue}
We performed joint training on the MNIST (CNN), CIFAR-10, STL-10, and Tiny ImageNet datasets. The architectures used for CIFAR-10, STL-10, and Tiny ImageNet are provided in Appendix \ref{app-cnnarc}. We used a batch size of 100 for the MNIST, CIFAR-10, and STL-10 datasets, and a batch size of 200 for the Tiny ImageNet dataset. For MNIST, we use the same architecture as for CIFAR-10. The complete set of hyperparameters for joint training is detailed in Tables \ref{tab:hypermnist-joint}, \ref{tab:hypercifar-joint}, \ref{tab:hyperstl-joint} and \ref{tab:hypertimage-joint}, corresponding to the MNIST, CIFAR-10, STL-10, and Tiny ImageNet datasets, respectively. 

For Tiny ImageNet, the first two layers are trained first, and their weights are then frozen while training the last three layers. This approach helps reduce the hyperparameter search space.

\begin{table*}[ht]
\centering
\caption{\textcolor{blue}{Hyperparameters for joint training on the MNIST (CNN) dataset.}}
\label{tab:hypermnist-joint}
\begin{threeparttable}
{\color{blue}
\begin{tabular}{lccccccccc}
\toprule
Layer %& \multicolumn{9}{c}{CIFAR-10} \\
%\cmidrule(lr){2-10} 
        & $lr$ & $\Theta_{\text{pos}}$ & $\Theta_{\text{neg}}$ & $\lambda$ & $w_d$ & $\gamma$ & $\text{Alg}$ & $\text{Dropout}$ & $\text{Epochs}$\\
\midrule
1     & 0.004     & 1     & 1    & 0    & 0.0003 & 0.7 & {$\/$} & - & 5\\
2 & 0.003     & 3     & 3    & 0    & 0.0003 &  0.7 & "2" & -  & 5 \\
3 & 0.0003     & 6     & 6    & 0 & 0.0003 &  0.7 & "2" & 0.2  & 5  \\
\bottomrule
\end{tabular}}
\end{threeparttable}
\end{table*}

\begin{table*}[ht]
\centering
\caption{\textcolor{blue}{Hyper-parameters for joint training on the CIFAR dataset.}}
\begin{threeparttable}
{\color{blue}
\begin{tabular}{lccccccccc}
\toprule
Layer %& \multicolumn{9}{c}{CIFAR-10} \\
%\cmidrule(lr){2-10} 
        & $lr$ & $\Theta_{\text{pos}}$ & $\Theta_{\text{neg}}$ & $\lambda$ & $w_d$ & $\gamma$ & $\text{Alg}$ & $\text{Dropout}$ & $\text{Epochs}$\\
\midrule
1     & 0.02     & 1     & 2    & 0.0008    & 0.0001 & 0.99 & {$\/$} & - & 6\\
2 & 0.001     & 2     & 5    & 0.0004    & 0.0003 & 0.9 & "1" & -  & 6 \\
3 & 0.0004     & 5     & 7    & 0.0016 & 0.0001 & 0.99 & "2" & 0.2  & 13  \\
\bottomrule
\end{tabular}
}
\end{threeparttable}
\label{tab:hypercifar-joint}
\end{table*}

\begin{table*}[ht]
\centering
\caption{\textcolor{blue}{Hyper-parameters for joint training on the STL-10 dataset.}}
\label{tab:hyperstl-joint}
{\color{blue}
\begin{tabular}{lccccccccc}
\toprule
Layer  %& \multicolumn{9}{c}{STL-10}\\
%\cmidrule(lr){2-10} 
        & $lr$ & $\Theta_{\text{pos}}$ & $\Theta_{\text{neg}}$ & $\lambda$ & $w_d$ & $\gamma$ & $\text{Alg}$ & $\text{Dropout}$ & $\text{Epochs}$ \\
\midrule
1   &  0.02     & 0     & 3    & 0 & 0.001 & 0.9 & {} & -  & 4\\
2   &0.001     & 4     & 5    & 0 & 0.001 & {0.99} & "2" & -  & 8 \\
3   &0.0004     & 7     & 8    & 0 & 0 & 0.9 & "2" & -  & 12\\
4   &0.0001     & 6     & 9    & 0 & 0.0003 & 1 & "2" & 0.6 & 21\\
\bottomrule
\end{tabular}}
\end{table*}

\begin{table*}[ht]
\centering
{\color{blue}
\caption{\textcolor{blue}{Hyper-parameters for joint training on the Tiny ImageNet dataset.}}
\label{tab:hypertimage-joint}
\begin{tabular}{lccccccccc}
\toprule
Layer  %& \multicolumn{9}{c}{STL-10}\\
%\cmidrule(lr){2-10} 
        & $lr$ & $\Theta_{\text{pos}}$ & $\Theta_{\text{neg}}$ & $\lambda$ & $w_d$ & $\gamma$ & $\text{Alg}$ & $\text{Dropout}$ & $\text{Epochs}$ \\
\midrule
1   &  0.011     & 0     & 1    & 0 & 0.001 & 0.9 & {} & -  & 6\\
2   &0.001     & 1     & 2    & 0 & {0.0003} & {0.8} & "1" & 0.1  & 15 \\
3   &0.00175     & 5     & 8    & 0 & 0 & 1 & "1" & -  & 17\\
4   &0.0002     & 5     & 9    & 0 & 0.001 & 0.99 & "2" & - & 19\\
5   &0.0003     & 3     & 7    & 0 & 0.0001 & 1 & "1" & 0.3 & 25\\
\bottomrule
\end{tabular}}
\end{table*}
%%%%%%%%%%%%%%%%%%%%%%%%%%%%%%%%%%%%%%%%%%%%%%%%%%%%%%%%%%%%%%%%%%%%%%%%%%%%%%%
%%%%%%%%%%%%%%%%%%%%%%%%%%%%%%%%%%%%%%%%%%%%%%%%%%%%%%%%%%%%%%%%%%%%%%%%%%%%%%%
\endgroup
\newpage
\section{Linear evaluation}
\label{app-lindout}

We utilize the same linear classifier as detailed in \cite{S2}. For vision tasks, the linear classifier employs a mini-batch size of 64 and is trained for 50 epochs on the MNIST, CIFAR-10, and for 100 epochs on the STL-10 dataset. \textcolor{blue}{For the Tiny ImageNet dataset, a mini-batch size of 256 is used, and the model is trained for 100 epochs.} The learning rate starts at 0.001 and is progressively halved at [20\%, 35\%, 50\%, 60\%, 70\%, 80\%, 90\%] of the total epochs. Data augmentation is applied to enhance model robustness, with random horizontal flipping used for CIFAR-10, and random cropping and flipping used for STL-10 \textcolor{blue}{and Tiny ImageNet}. For FSDD dataset, the linear classifier employs a mini-batch size of 1 and is trained for 10 epochs. The learning rate starts at 0.0005 and is progressively halved at [20\%, 35\%, 50\%, 60\%, 70\%, 80\%, 90\%] of the total epochs.

\begin{comment}
\begin{table*}[ht]
\centering
\caption{Comparison of SCFF and SoftHebb methods across different layers for CIFAR dataset.}
\begin{tabular}{lcccccc}
\toprule
Methods & \multicolumn{2}{c}{1 layer} & \multicolumn{2}{c}{2 layers} & \multicolumn{2}{c}{3 layers} \\
\cmidrule(lr){2-3} \cmidrule(lr){4-5} \cmidrule(lr){6-7}
        & \#neurons & accuracy & \#neurons & accuracy & \#neurons & accuracy \\
\midrule
SCFF     & 6144     & 72.2     & 12288    & 78.5     & 18432    & 80.6 \\
SoftHebb & 24576    & 71.1     & 24576    & 77.7     & 24576    & 80.3 \\
\bottomrule
\end{tabular}
\label{compsofthebb}
\end{table*}    
\end{comment}

%\newpage
\section{Hierarchical representations}
\label{app-hierach}
In Appendix \ref{app-hierach}, we delve into the concept of hierarchical representations in convolutional neural networks (CNNs), specifically as learned by SCFF method on the STL-10 dataset. Fig. \ref{figs:heatmap} illustrates this concept by showcasing Class Activation Maps (CAMs) generated by a neural network after different stages of convolutional layers. The CAMs were calculated using the torchcam package \cite{S4}, which allows us to visualize the regions of an image that most significantly influence the network's decision.

The progression of CAMs from Layer 1 to Layer 4 demonstrates how the network increasingly abstracts the features it learns from the input images. In Layer 1, the network focuses on low-level features such as edges and textures, while by Layer 4 (combined with layer 3), it has learned to identify more complex and abstract features that are crucial for accurate classification. Warmer colors in the CAMs (e.g., red and yellow) indicate areas of higher relevance, showing how the network's focus shifts and intensifies on the most critical parts of the image as it moves through the layers. This hierarchical feature extraction underscores the effectiveness of the SCFF method in training CNNs, enabling them to capture the intricate details necessary for tasks like image recognition and classification.

\begin{figure*}[ht]
%\vskip 0.2in
\begin{center}
\includegraphics[width=1\textwidth, clip=true, trim=2 2 2 2]{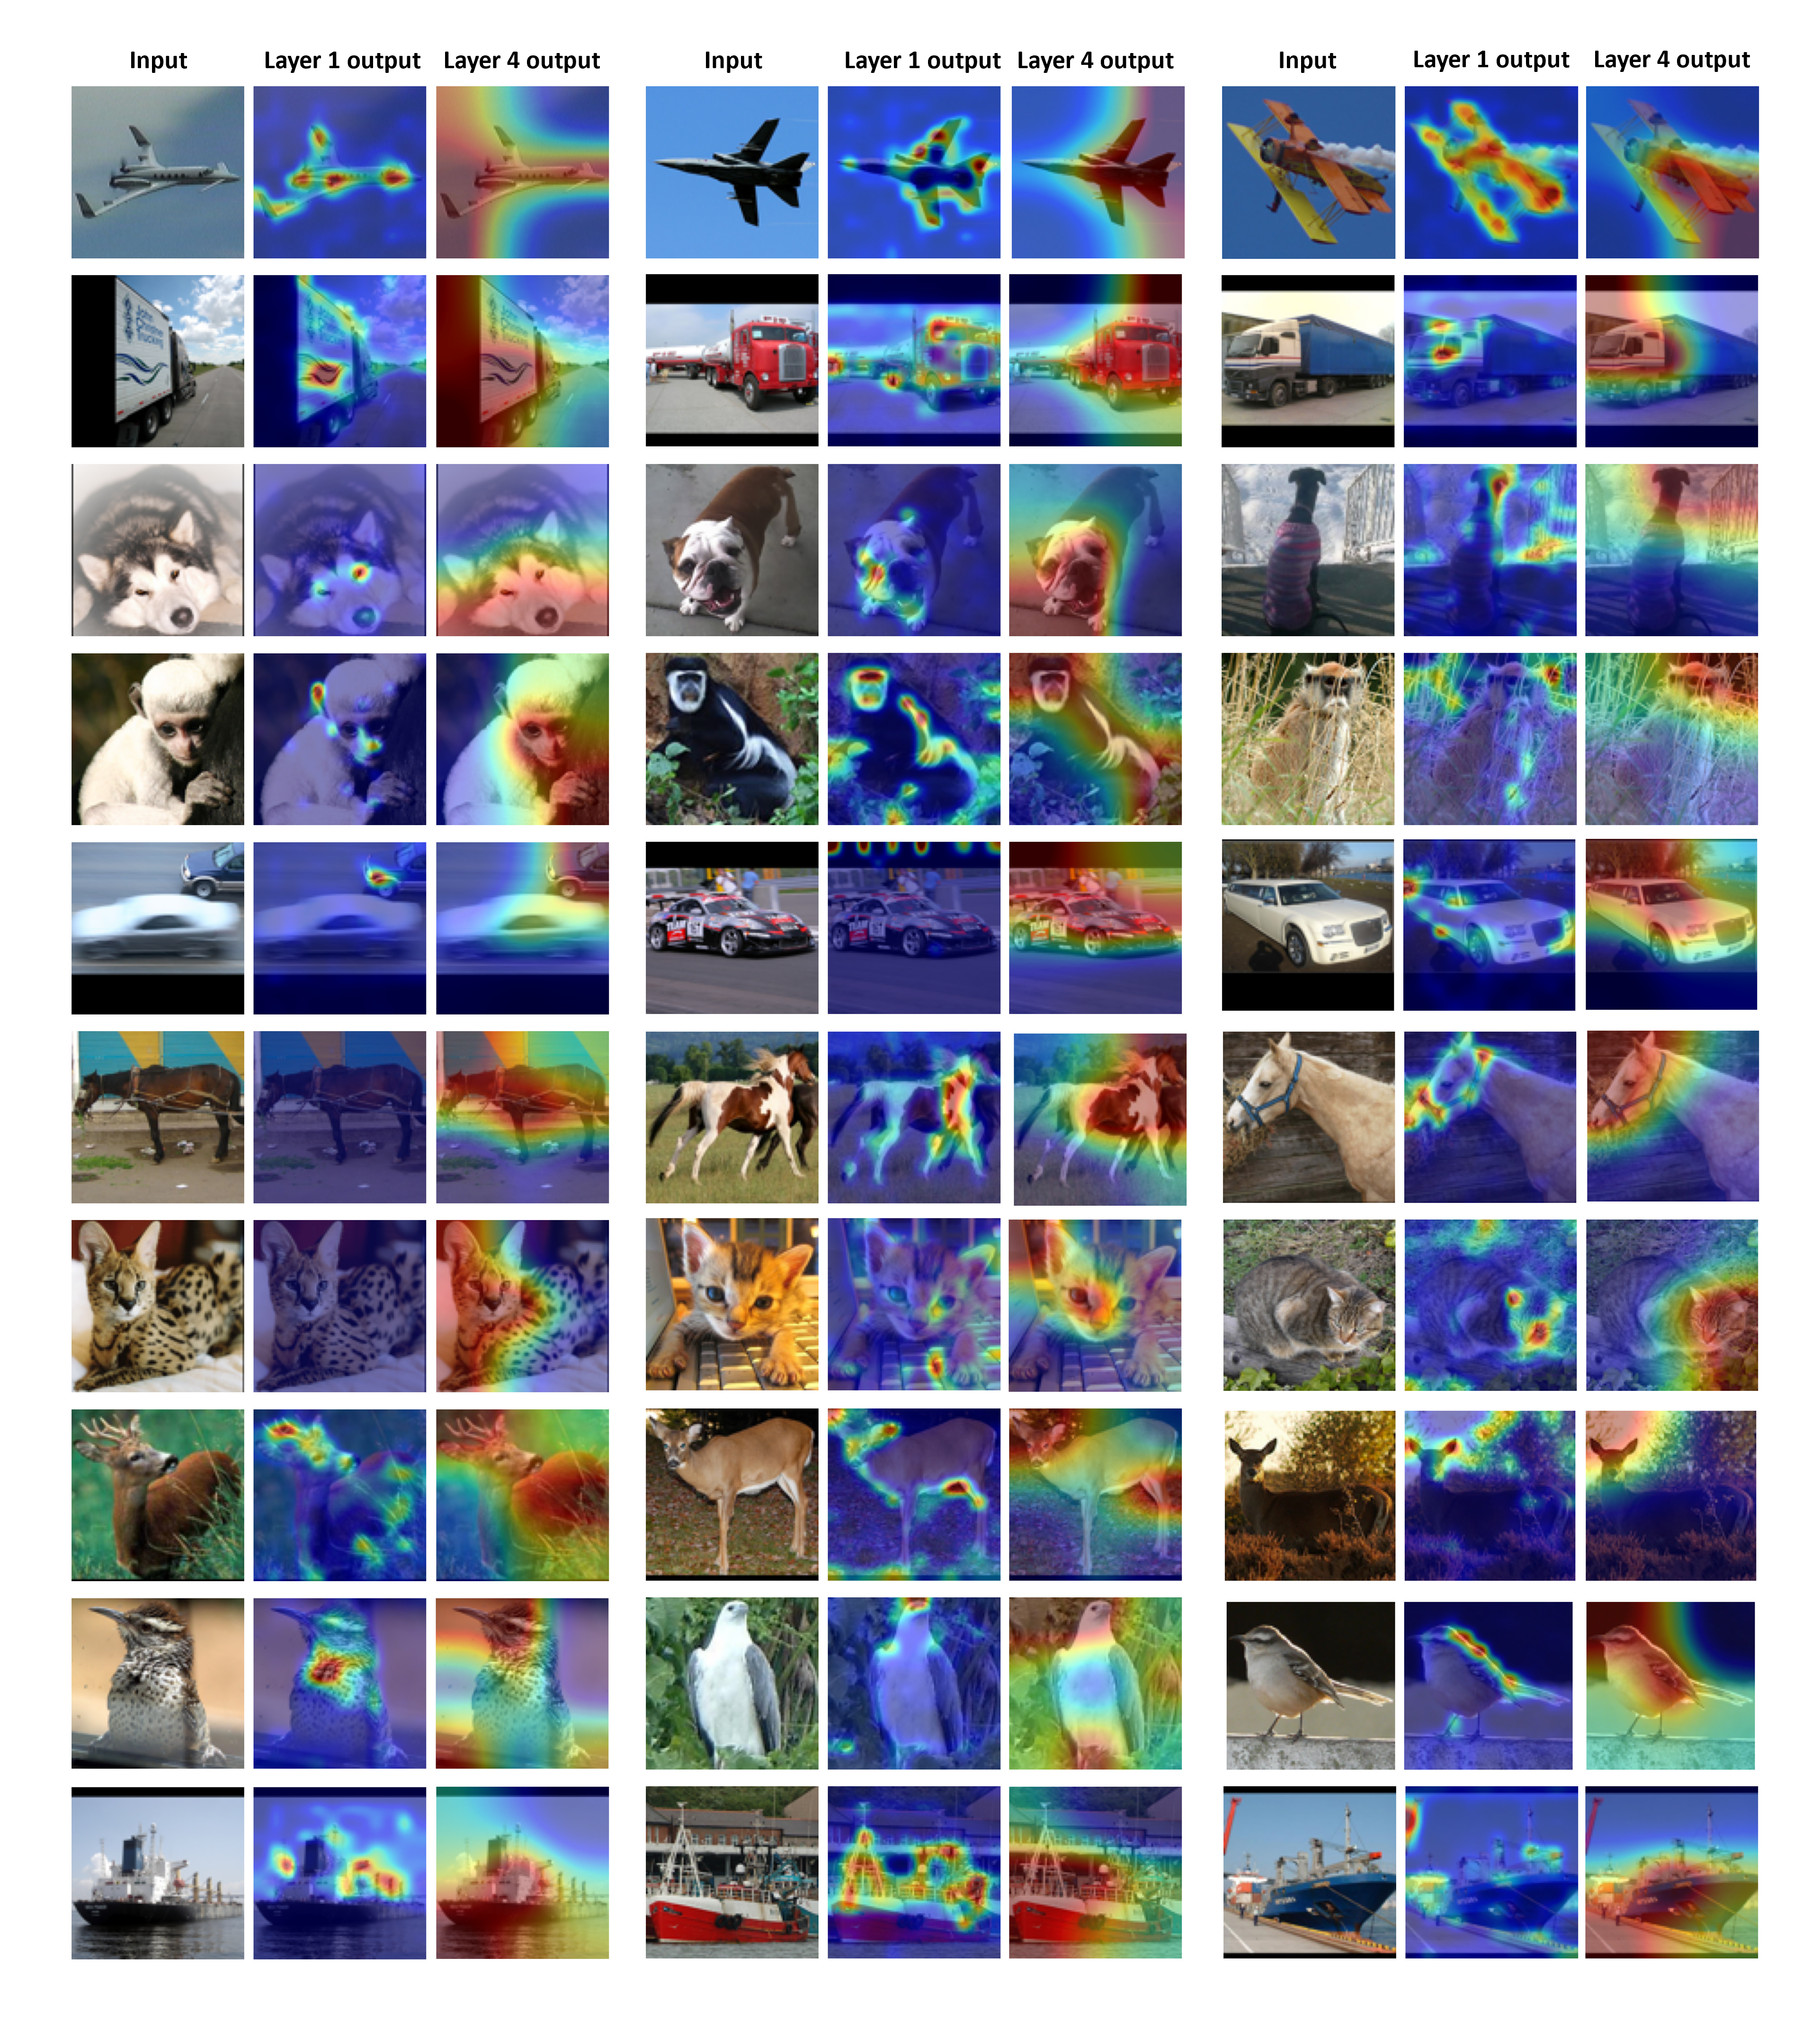}
\caption{Indications for hierarchical representations learned by SCFF on STL-10 dataset. The "input" columns show the original input images to the network. The "Layer 1 output" and "Layer 4 output" columns display Class Activation Maps (CAMs) generated by the trained neural network after 1 convolutional layer and after 4 convolutional layers (combined with layer 3's features), respectively. These heatmaps highlight the regions in the image that contributed most strongly to the network's decision, with warmer colors (e.g., red and yellow) indicating areas of higher relevance. This progression demonstrates the increasingly abstract feature representations learned at deeper network layers.}
\label{figs:heatmap}
\end{center}
%\vskip -0.2in
\end{figure*}

% Manually include appendix bibliography
%\section*{References for Appendix}
%\nocite{*}  % Include all entries from bib-ap.bib
%\bibliography{bib-ap}  % Use a separate .bib file for the appendix references
\end{appendices}

\clearpage

%\bibliographystyle{plain}  % or any 
%\bibliography{bib-ap}

\end{document}
